# Supplementary material for: Graph Structure Learning with Bi-level Optimization
Source: arXiv:2411.17062 source file (2024-11-26)
Supplement: Supplementary file 1 [file Appendix.tex]

\subsection{Unifying Various GNN and Beyond}
To extend the graph convolution operator to the most existing graph convolutions, we reformulate the classical GNN model into a unified form.
\paragraph{GCN}
The forward propagation of GCN is formulated as follows:
\begin{equation}
  \label{gcn}
  \bm{H}^{(l)}=\sigma(\tilde{\bm{D}}^{-\frac{1}{2}}\tilde{\bm{A}} \tilde{\bm{D}}^{-\frac{1}{2}}\bm{H}^{(l-1)}\bm{W}), \notag
\end{equation} 
where $\bm{H}^{(0)}=\bm{X}$, $\tilde{\bm{A}}=\bm{A}+\bm{I}$, $\tilde{\bm{D}}_{nn}=\sum_i\tilde{\bm{A}}_{ni}$,
$\bm{W} \in \mathbb{R}^{D \times C}$ is the trainable parameters, $\bm{I}$ denotes the identity matrix, $\sigma$ is a nonlinear function.
For better understanding of the propagation of GCN, 
we rewrite the embedding update in the following form,
\begin{equation}
  \begin{aligned}
  &\bm{h}_v^{(l)}=\sum_{u \in \mathcal{N}(v)+v}\frac{1}{\sqrt{d_v}\sqrt{d_u}}\bm{W}^{(l-1)}\bm{h}_v^{(l-1)},\\
  \bm{H}&^{(l)}=\sigma_1(\sigma_2(\bm{Z})\odot(\tilde{\bm{A}}))^{(l-1)}\bm{H}^{(l-1)}\bm{W}^{(l-1)}),\\
  % &=\sigma((\bm{Z}^{(l-1)}\odot\tilde{\bm{A}})\bm{H}^{(l-1)}\bm{W}^{(l-1)}),\\
  \bm{Z}_{ij}&=\frac{1}{\sqrt{d_i}\sqrt{d_j}}\ \ \ where \ \ \tilde{\bm{A}}_{ij}=1,\ and \ j\in \mathcal{N}(i),\notag
  \end{aligned}
\end{equation}
where $\bm{W}^{(l)}$ is the trainable parameters on $l$-th layer, $\sigma_1$ is the activate function, such as $ReLU$,
$\sigma_2=\textit{min[max[0,x],1]}$ is the a non-negative activation function. 

\paragraph{GAT}
GAT assigns different weights to each neighbor node, and update the node embeddings with weighted average of neighbors:
% The formulation of Eq. \ref{GAT} can be rewritten as
\begin{equation}
  \begin{aligned}
  \bm{H}^{(l)}&
  % \sigma(\frac{1}{K}\sum_{k=1}^K((\bm{U}({\tilde{\bm{A}}}))^{(l-1)}_k\bm{H}^{(l-1)}\bm{W}_k^{(l-1)}))\\
  =\sigma_1(\frac{1}{K}\sum_{k=1}^K((\sigma_2(\bm{Z}_k)\odot\tilde{\bm{A}})\bm{H}^{(l-1)}\bm{W}_k^{(l-1)})),\\
  \bm{Z}_{k,ij}=&Softmax(atten(\bm{W}_k^{(l-1)}\bm{h}^{(l-1)}_i,\bm{W}_k^{(l-1)}\bm{h}^{(l-1)}_{j}))\\
  &\ \ \ where \ \ \tilde{\bm{A}}_{ij}=1, \ and \ j\in \mathcal{N}(i),\notag
  \end{aligned}
\end{equation}
where $\bm{W}^{(l-1)}_k$ is the parameter of $k$th multi-head attention on $(l-1)$th layer, 
$Softmax$ is the Softmax operation and $atten$ is the self-attention operation. 

\paragraph{GraphSAGE}
The GraphSAGE is one representative of the spatial approaches, 
which learns how to aggregate feature information from a node’s local neighborhood, and the reformulate is as follows:
\begin{equation}
  \begin{aligned}
  \bm{H}^{(l)}
  % &=\sigma(Concat(\bm{H}^{(l-1)},(\bm{U}({\bm{A}}))^{(l-1)}\bm{H}^{(l-1)})\bm{W}^{(l-1)}),\\
  &=\sigma_1(Concat(\bm{H}^{(l-1)},(\sigma_2(\bm{Z})\odot{\bm{A}})\bm{H}^{(l-1)})\bm{W}^{(l-1)}),\\
  &\ \ \  \bm{Z}_{ij}^{(l-1)}=\frac{1}{d_i}\ \ \ where \ \ \bm{A}_{ij}=1,\ and \ j\in \mathcal{N}(i).\notag
  \end{aligned}
\end{equation}
% where $Concat$ is the concatenation operation. 

\paragraph{JK-Net}
JK-Net learns the node representation form deep layers by jumping network.
There exists different ways to aggregate features from different layers, we take the concatenation as an example in our work (other aggregation methods are also applicable).
The formulation of JK-Net is as follows:
% The matrix representation of node update for JK-Net is 
\begin{equation}
  \begin{aligned}
  \bm{H}^{(L)}&
  =FC(Concat(\bm{H}^{(0)},\bm{H}^{(1)},\cdots,\bm{H}^{(L-1)}))\\
  wi&th \; \bm{H}^{(l)}=\sigma_1((\sigma_2(\bm{Z})\odot{\tilde{\bm{A}}})\bm{H}^{(l-1)}\bm{W}^{(l)},\\
%   =FC(Concat(\sigma_1((\sigma_2(\bm{Z})\odot{\tilde{\bm{A}}})\bm{H}^{(L-1:0)}\bm{W}^{(L-1:0)}))),\\
  \bm{Z}_{ij}&=\frac{1}{\sqrt{d_id_j}}\ \ \ where \ \ \tilde{\bm{A}}_{ij}=1,\ and \ j\in \mathcal{N}(i),\notag
  \end{aligned}
\end{equation}
where $FC$ is a fully connect layer, and $Concat$ is the concatenation operation. .

\section{Updating of outer parameters}
We optimize the outer parameters $\bm{Z}$ by fixing the inner parameters $\bm{\mathcal{W}}_1,\cdots,\bm{\mathcal{W}}_\tau$.
Formally, the derivative of the outer objective to the hyperparameter $\bm{Z}$ (hypergradient) is formulated as
\begin{equation}
  \nabla_{\bm{Z}}F(\bm{\mathcal{W}}^*(\bm{Z}))=\\
  \partial_{\bm{\mathcal{W}}}F(\bm{\mathcal{W}}^*(\bm{Z}))\nabla_{\bm{Z}}\\
  \bm{\mathcal{W}}^*(\bm{Z})+\partial_{\bm{Z}}F(\bm{\mathcal{W}}^*(\bm{Z})).\notag
\end{equation}
\begin{equation}
  \label{update}
  \bm{Z}=\bm{Z}-\eta_{o}\nabla_{\bm{Z}}\bm{F}(\bm{\mathcal{W}}_{\bm{Z},\tau},\bm{Z}).
\end{equation}
The parameter of outer optimization $\bm{Z}$ is updated with the parameters of $\bm{\mathcal{W}}_1,\cdots,\bm{\mathcal{W}}_\tau$.
The details of updating $\bm{Z}$ is shown on line 8-11 in $\textbf{Algorithm}$ 1.
For $t=\tau$ downto 1, we define the matrices
\begin{equation}
  \begin{aligned}
 &\bm{\alpha}_t=\left\{
  \begin{aligned}
  &\nabla F(\bm{\mathcal{W}}_n)\qquad\qquad\qquad \ \ \ \ if\  n=\tau \\
  &\nabla F(\bm{\mathcal{W}}_n)\bm{M}_{\tau}\cdots \bm{M}_{n+1}\quad if\ n=1,\cdots,\tau-1
  \end{aligned}
 \right.\notag\\
\end{aligned}
\end{equation}
with
\begin{equation}
%   \begin{aligned}
    \bm{M}_n=\frac{\partial \bm{\mathcal{W}}_n}{\partial \bm{\mathcal{W}}_{n-1}},\;
    \bm{N}_n=\frac{\partial \bm{\mathcal{W}}_n}{\partial \bm{Z}},\notag
%   \end{aligned}
\end{equation}
and the update of $\bm{Z}$ can be formulated as
\begin{equation}
\label{outer}
\begin{aligned}
  \nabla_{\bm{Z}}F(\bm{\mathcal{W}}^*(\bm{Z}))&=\nabla_{\bm{Z}} F(\bm{\mathcal{W}}_{\tau})\sum_{r=1}^{\tau}(\prod_{s=r+1}^{\tau}\bm{M}_s)\bm{N}_r,\\
  \bm{Z}=\bm{Z}&-\eta_{o}\nabla_{\bm{Z}}F(\bm{\mathcal{W}}^*(\bm{Z})).
  \end{aligned}
\end{equation}

\section{Defeating of over fitting}

\section{Visualization}
 \begin{figure}
%  \vspace{-2cm}
  \centering
  \setlength{\abovecaptionskip}{0cm}
  \setlength{\belowcaptionskip}{0cm}
  \includegraphics[scale=0.455]{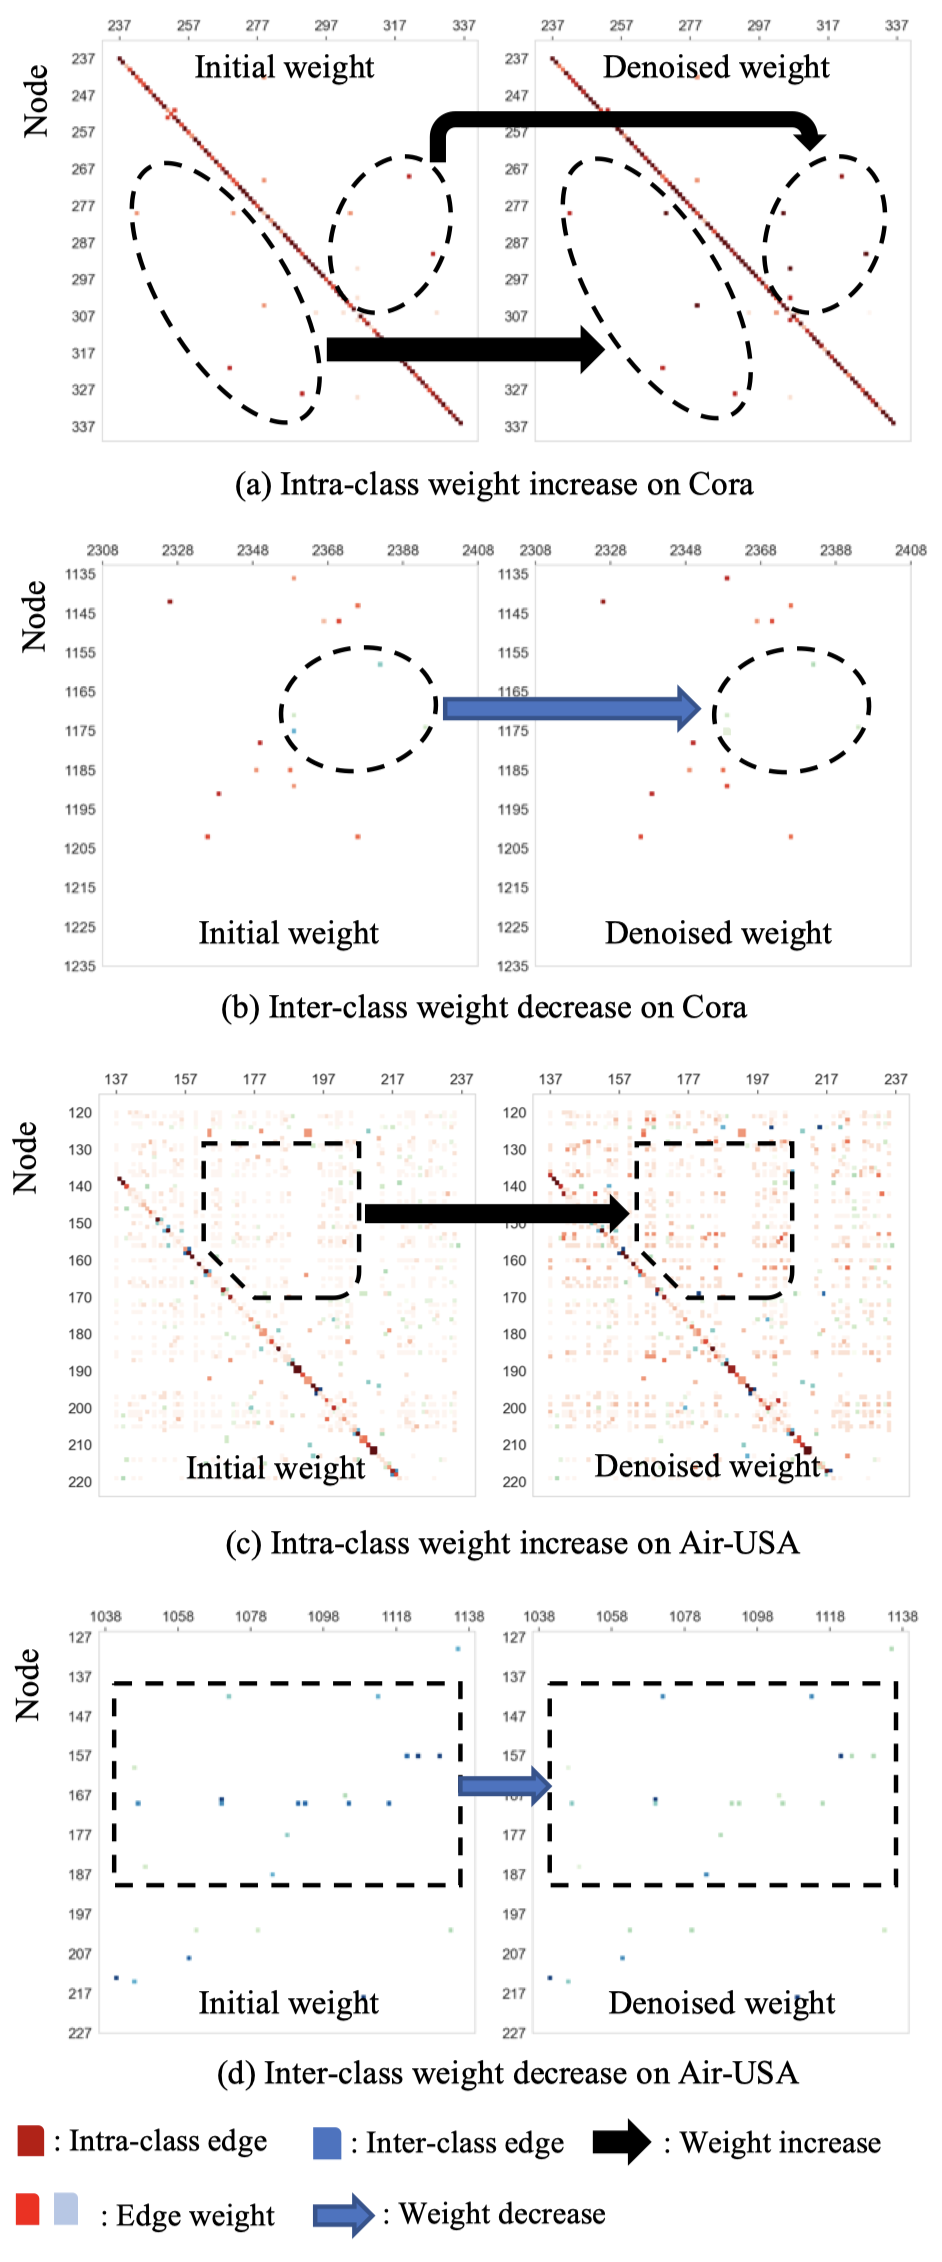}
%   \captionsetup{justification=centering}
  \caption{Comparison of initial weight and denoised weight to visualize the effect of denoising.}
%   \vspace{-2cm}
  \label{denoise}
\end{figure}

To investigate the effect of the connection strength matrix $\bm{Z}$, we further visually compare the initialization of $\bm{Z}$ (\ie initial weight) and its value after optimization (\ie denoised weight).
As both of them are large and sparse matrix, we visualize part of the denoised weight with a region of $100\times{100}$,
which is shown on Figure \ref{denoise}. 
We show the results on Core and Air-USA where the improvement of UGSL is the smallest and largest, respectively.
In the figures, we use read pixels and blue pixels to represent intra-class and inter-class edges respectively, where deeper color represents larger values.
From Figure \ref{denoise}(a) and (b), we find that the denoised weight matrix mainly decreases the value corresponds to inter-class connections, which thus can downweight the corresponds neighbor during representation propagation. In some cases, the denoised weight increases the weight of intra-class connections, which also facilitates denoising.
Apparently, most edges in Air-USA are intra-class, and UGSL still downweights a portion of inter-class edges and increases the intra-class weights as shown in Figure~\ref{denoise}(c) and (d). This is because the denoised weight is learned towards the overall classification objective. 

\section{Hyperparametric Analysis}
%\paragraph{Ablation experiment.}
%\label{ablation_exp}

\begin{figure}
  \centering
  \setlength{\abovecaptionskip}{0cm}
  \setlength{\belowcaptionskip}{0cm}
  \includegraphics[scale=0.33]{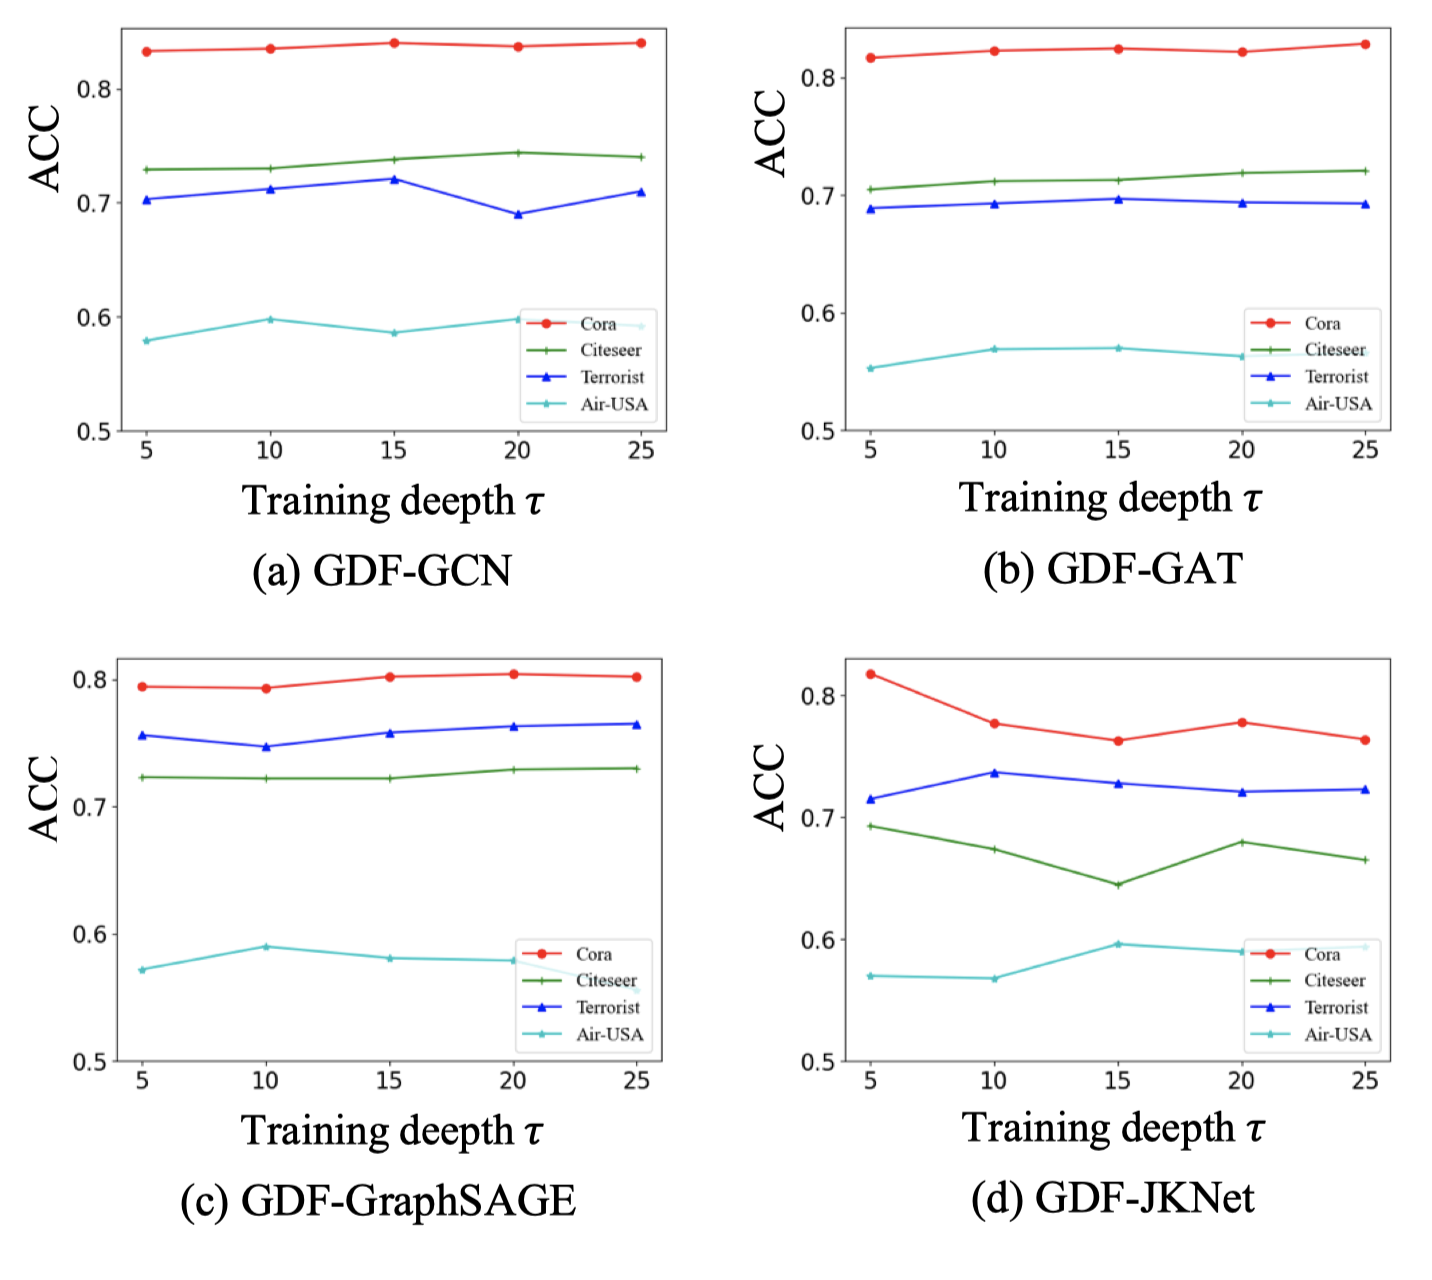}
  \caption{The performance of UGSL on the four datasets as changing the value of $\tau$ from 5 to 25.}
%   \vspace{-0.4cm}
  \label{ablation}
\end{figure}

We then investigate how the hyperparameters of UGSL affect its effectiveness. As introduced in Sec. \ref{UDF}, the most critical hyperparameter of UGSL is the training depth of inner optimization step (\ie $\tau$), which also is the number of gradient update in each inner optimization step. For the consideration of computing cost, we cap the value of $\tau$ at 25 and changes its value with step of 5, \ie setting $\tau \in \{5,10,15,20,25\}$.

Figure \ref{ablation} shows the performance of UGSL applied to the four classical GNN architectures on the four datasets as changing the value of $\tau$.
From the figures, we have the following observations: (1) in most cases, the overall performance of the proposed UGSL on each dataset is relatively stable as increasing the value of $\tau$. This result indicates the insensitivity of UGSL to the hyperparameter.
(2) While increasing the value of $\tau$ can slightly improve the performance of UGSL, we still suggest setting it as a relatively small value. This is because enlarging $\tau$ will increase the memory and computation cost of UGSL.

\section{Datasets}

\begin{table}
  \small
    \caption{Summary statistics for the datasets.}
    % \vspace{-0.3cm}
    \label{data}
    \centering
    \begin{tabular}{lcccc}
      \toprule
      \multicolumn{1}{c}{}&\multicolumn{1}{c}{Cora}&\multicolumn{1}{c}{Citeseer}&\multicolumn{1}{c}{Terrorist}&\multicolumn{1}{c}{Air-USA} \\
      \cmidrule(r){1-5}
      Nodes              &2,708     &3,327      &1,293    &1,190        \\
      Edges              &5,278     &4,552      &3,172    &13,599      \\
      Inter ratio        &0.151     &0.194     &0.362    &0.289        \\
      Features           &1,433     &3,703      &106      &238        \\
      Class              &7         &6          &6        &4          \\
      Training set         &140       &120        &129      &119           \\
      Validation set       &500       &500        &258      &238      \\
      Testing set               &1,000     &1,000      &906      &833         \\
      \bottomrule
    \end{tabular}
    % \vspace{-0.2cm}
  \end{table}
